# Supplementary material for: Measurements of the Most Significant Software Security Weaknesses
Source: arXiv:2104.05375 source file (2021-04-12)
Supplement: Supplementary file 1 [file Appendix.tex]

\begin{appendix}
\label{appendix}

%\clearpage

\section{Appendix: Supplementary Table from Outside Source}
\input{MITRETop25CWE}

\end{appendix}
